# Supplementary material for: Unifying Tracking and Image-Video Object Detection
Source: arXiv:2211.11077 source file (2023-11-19)
Supplement: Supplementary file 1 [file det_arxiv.tex]

\begin{figure}[h]
%\vspace{0.2cm}
\begin{center}
%\hspace*{-0.55cm}  
\captionsetup{type=figure}
\resizebox{1.\linewidth}{!}{
	\begin{tikzpicture}
		\tikzstyle{myarrows}=[line width=0.6mm,draw=blue!50,-triangle 45,postaction={draw, line width=0.05mm, shorten >=0.01mm, -}]
		\tikzstyle{mylines}=[line width=0.6mm]
		% Main size box
		%\draw[thin, color = black] (10, -5) -- (-10, -5) -- (-10, 5) -- (10, 5) -- (10, -5); 
		 
   		% Denotations location control
		\pgfmathsetmacro{\dx}{3.65} 
		\pgfmathsetmacro{\dy}{2}

		\node at (-4-\dx, -6.5+3.65*\dy){\texttt{COCO}~\cite{lin2014coco}};
		\node at (-4, -6.5+3.65*\dy){\texttt{VID}~\cite{russakovsky2015vid}};
		\node at (-4+\dx, -6.5+3.65*\dy){\texttt{MOT17}~\cite{Milan2016MOT16AB}};

		\node at (-4-\dx, -6.5+3*\dy) {\includegraphics[width=3.5cm]{fig/COCO/91-341681-3_3.png}};  
		\node at (-4-\dx, -6.5+2*\dy) {\includegraphics[width=3.5cm]{fig/COCO/14-51712-2_2.png}}; 
		\node at (-4-\dx, -6.5+1*\dy) {\includegraphics[width=3.5cm]{fig/COCO/2346.png}};  
		\node at (-4-\dx, -6.5) {\includegraphics[width=3.5cm]{fig/COCO/144.png}}; 
		\node at (-4-\dx, -6.5-\dy) {\includegraphics[width=3.5cm]{fig/COCO/54592.png}}; 
		\node at (-4-\dx, -6.5-2*\dy) {\includegraphics[width=3.5cm]{fig/COCO/66771.png}}; 
		\node at (-4-\dx, -6.5-3*\dy) {\includegraphics[width=3.5cm]{fig/COCO/214753.png}}; 
		\node at (-4-\dx, -6.5-4*\dy) {\includegraphics[width=3.5cm]{fig/COCO/230008.png}};

		%\node at (-4, -6.5+3*\dy) {\includegraphics[width=3.5cm]{fig/VID/5403.jpg}}; 
		\node at (-4, -6.5+3*\dy) {\includegraphics[width=3.5cm]{fig/VID/1506.png}}; 
		\node at (-4, -6.5+2*\dy) {\includegraphics[width=3.5cm]{fig/VID/antelope2.png}};  
		\node at (-4, -6.5+1*\dy) {\includegraphics[width=3.5cm]{fig/VID/3399.png}};  
		\node at (-4, -6.5) {\includegraphics[width=3.5cm]{fig/VID/3918.png}}; 
		\node at (-4, -6.5-\dy) {\includegraphics[width=3.5cm]{fig/VID/4268.png}}; 
		\node at (-4, -6.5-2*\dy) {\includegraphics[width=3.5cm]{fig/VID/3635.png}}; 
		\node at (-4, -6.5-3*\dy) {\includegraphics[width=3.5cm]{fig/VID/antelope.png}}; 
		\node at (-4, -6.5-4*\dy) {\includegraphics[width=3.5cm]{fig/VID/5403.png}};

		\node at (-4+\dx, -6.5+3*\dy) {\includegraphics[width=3.5cm]{fig/MOT-detect/2536.png}}; 
		\node at (-4+\dx, -6.5+2*\dy) {\includegraphics[width=3.5cm]{fig/MOT-detect/550.png}}; 
		\node at (-4+\dx, -6.5+1*\dy) {\includegraphics[width=3.5cm]{fig/MOT-detect/2408.png}};  
		\node at (-4+\dx, -6.5) {\includegraphics[width=3.5cm]{fig/MOT-detect/2480.png}};  
		\node at (-4+\dx, -6.5-\dy) {\includegraphics[width=3.5cm]{fig/MOT-detect/2500.png}};  
		\node at (-4+\dx, -6.5-2*\dy) {\includegraphics[width=3.5cm]{fig/MOT-detect/228.png}};  
		\node at (-4+\dx, -6.5-3*\dy) {\includegraphics[width=3.5cm]{fig/MOT-detect/2578.png}};  
		\node at (-4+\dx, -6.5-4*\dy) {\includegraphics[width=3.5cm]{fig/MOT-detect/998.png}};

	\end{tikzpicture}
	}  
	\vspace*{-0.7cm}
    \caption{\texttt{TrIVD}'s object detection results on \texttt{COCO}, \texttt{VID}, and \texttt{MOT17}. With multi-dataset co-training, \texttt{TrIVD} detects objects (e.g., traffic lights, bicycles, motorcycles) not annotated by \texttt{MOT17}~($3^{\text{rd}}$ column).}
	 \label{app_fig: det}
\end{center}
\end{figure}
