# Supplementary material for: Unifying Tracking and Image-Video Object Detection
Source: arXiv:2211.11077 source file (2023-11-19)
Supplement: Supplementary file 2 [file mot_a_arxiv.tex]

\begin{figure*}[t]
\vspace{-1.3cm}
\begin{center}
%\hspace*{-0.7cm}  
\captionsetup{type=figure}
\resizebox{0.95\linewidth}{!}{
	\begin{tikzpicture}
		\tikzstyle{myarrows}=[line width=0.6mm,draw=blue!50,-triangle 45,postaction={draw, line width=0.05mm, shorten >=0.01mm, -}]
		\tikzstyle{mylines}=[line width=0.6mm]
		% Main size box
		%\draw[thin, color = black] (10, -5) -- (-10, -5) -- (-10, 5) -- (10, 5) -- (10, -5); 
		 
   		% Global location control
		\pgfmathsetmacro{\dx}{3.6} 
		\pgfmathsetmacro{\dy}{2}
		
		\node at (-4-5.55*\dx, -6.5+9.65*\dy){\color{cb!90}$\mathbf{t}$};
		\draw [-to, line width=0.6mm, color = cb] (-4-5.55*\dx, -6.5+9.48*\dy) -- (-4-5.55*\dx, -6.5-0.51*\dy); 
		
		\node at (-4-5*\dx, -6.5+9.65*\dy){\small\textbf{\color{cb}Track} \textit{``airplane''}};
		\node at (-4-4*\dx, -6.5+9.65*\dy){\small\textbf{\color{cb}Track} \textit{``bird''}};
		\node at (-4-3*\dx, -6.5+9.65*\dy){\small\textbf{\color{cb}Track} \textit{``giant panda''}};
		\node at (-4-2*\dx, -6.5+9.65*\dy){\small\textbf{\color{cb}Track} \textit{``car''}};

		% airplane 1
		\node at (-4-5*\dx, -6.5+9*\dy) {\includegraphics[width=3.5cm]{sub/appendix/fig/airplane1/000000.JPEG}}; 
		\node at (-4-5*\dx, -6.5+8*\dy) {\includegraphics[width=3.5cm]{sub/appendix/fig/airplane1/000016.JPEG}}; 
		\node at (-4-5*\dx, -6.5+7*\dy) {\includegraphics[width=3.5cm]{sub/appendix/fig/airplane1/000030.JPEG}}; 
		\node at (-4-5*\dx, -6.5+6*\dy) {\includegraphics[width=3.5cm]{sub/appendix/fig/airplane1/000045.JPEG}}; 
		\node at (-4-5*\dx, -6.5+5*\dy) {\includegraphics[width=3.5cm]{sub/appendix/fig/airplane1/000056.JPEG}}; 
		\node at (-4-5*\dx, -6.5+4*\dy) {\includegraphics[width=3.5cm]{sub/appendix/fig/airplane1/000065.JPEG}}; 
		\node at (-4-5*\dx, -6.5+3*\dy) {\includegraphics[width=3.5cm]{sub/appendix/fig/airplane1/000076.JPEG}}; 
		\node at (-4-5*\dx, -6.5+2*\dy) {\includegraphics[width=3.5cm]{sub/appendix/fig/airplane1/000086.JPEG}}; 
		\node at (-4-5*\dx, -6.5+1*\dy) {\includegraphics[width=3.5cm]{sub/appendix/fig/airplane1/000105.JPEG}}; 
		\node at (-4-5*\dx, -6.5) {\includegraphics[width=3.5cm]{sub/appendix/fig/airplane1/000127.JPEG}};

		% birds
		\node at (-4-4*\dx, -6.5+9*\dy) {\includegraphics[width=3.5cm]{sub/appendix/fig/birds/000000.JPEG}}; 
		\node at (-4-4*\dx, -6.5+8*\dy) {\includegraphics[width=3.5cm]{sub/appendix/fig/birds/000081.JPEG}}; 
		\node at (-4-4*\dx, -6.5+7*\dy) {\includegraphics[width=3.5cm]{sub/appendix/fig/birds/000124.JPEG}}; 
		\node at (-4-4*\dx, -6.5+6*\dy) {\includegraphics[width=3.5cm]{sub/appendix/fig/birds/000167.JPEG}}; 
		\node at (-4-4*\dx, -6.5+5*\dy) {\includegraphics[width=3.5cm]{sub/appendix/fig/birds/000177.JPEG}}; 
		\node at (-4-4*\dx, -6.5+4*\dy) {\includegraphics[width=3.5cm]{sub/appendix/fig/birds/000190.JPEG}}; 
		\node at (-4-4*\dx, -6.5+3*\dy) {\includegraphics[width=3.5cm]{sub/appendix/fig/birds/000197.JPEG}}; 
		\node at (-4-4*\dx, -6.5+2*\dy) {\includegraphics[width=3.5cm]{sub/appendix/fig/birds/000207.JPEG}}; 
		\node at (-4-4*\dx, -6.5+1*\dy) {\includegraphics[width=3.5cm]{sub/appendix/fig/birds/000232.JPEG}}; 
		\node at (-4-4*\dx, -6.5) {\includegraphics[width=3.5cm]{sub/appendix/fig/birds/000257.JPEG}};

		% pandas
		\node at (-4-3*\dx, -6.5+9*\dy) {\includegraphics[width=3.5cm]{sub/appendix/fig/pandas/000000.JPEG}}; 
		\node at (-4-3*\dx, -6.5+8*\dy) {\includegraphics[width=3.5cm]{sub/appendix/fig/pandas/000016.JPEG}}; 
		\node at (-4-3*\dx, -6.5+7*\dy) {\includegraphics[width=3.5cm]{sub/appendix/fig/pandas/000044.JPEG}}; 
		\node at (-4-3*\dx, -6.5+6*\dy) {\includegraphics[width=3.5cm]{sub/appendix/fig/pandas/000058.JPEG}}; 
		\node at (-4-3*\dx, -6.5+5*\dy) {\includegraphics[width=3.5cm]{sub/appendix/fig/pandas/000091.JPEG}}; 
		\node at (-4-3*\dx, -6.5+4*\dy) {\includegraphics[width=3.5cm]{sub/appendix/fig/pandas/000094.JPEG}}; 
		\node at (-4-3*\dx, -6.5+3*\dy) {\includegraphics[width=3.5cm]{sub/appendix/fig/pandas/000115.JPEG}}; 
		\node at (-4-3*\dx, -6.5+2*\dy) {\includegraphics[width=3.5cm]{sub/appendix/fig/pandas/000140.JPEG}}; 
		\node at (-4-3*\dx, -6.5+1*\dy) {\includegraphics[width=3.5cm]{sub/appendix/fig/pandas/000164.JPEG}}; 
		\node at (-4-3*\dx, -6.5) {\includegraphics[width=3.5cm]{sub/appendix/fig/pandas/000191.JPEG}};

		% car
		\node at (-4-2*\dx, -6.5+9*\dy) {\includegraphics[width=3.5cm]{sub/appendix/fig/car/000000.JPEG}}; 
		\node at (-4-2*\dx, -6.5+8*\dy) {\includegraphics[width=3.5cm]{sub/appendix/fig/car/000012.JPEG}}; 
		\node at (-4-2*\dx, -6.5+7*\dy) {\includegraphics[width=3.5cm]{sub/appendix/fig/car/000019.JPEG}}; 
		\node at (-4-2*\dx, -6.5+6*\dy) {\includegraphics[width=3.5cm]{sub/appendix/fig/car/000030.JPEG}}; 
		\node at (-4-2*\dx, -6.5+5*\dy) {\includegraphics[width=3.5cm]{sub/appendix/fig/car/000037.JPEG}}; 
		\node at (-4-2*\dx, -6.5+4*\dy) {\includegraphics[width=3.5cm]{sub/appendix/fig/car/000042.JPEG}}; 
		\node at (-4-2*\dx, -6.5+3*\dy) {\includegraphics[width=3.5cm]{sub/appendix/fig/car/000047.JPEG}}; 
		\node at (-4-2*\dx, -6.5+2*\dy) {\includegraphics[width=3.5cm]{sub/appendix/fig/car/000055.JPEG}}; 
		\node at (-4-2*\dx, -6.5+1*\dy) {\includegraphics[width=3.5cm]{sub/appendix/fig/car/000067.JPEG}}; 
		\node at (-4-2*\dx, -6.5) {\includegraphics[width=3.5cm]{sub/appendix/fig/car/000092.JPEG}};

	\end{tikzpicture}
	}  
	\vspace*{-0.4cm}
    \caption{Visualizations on \texttt{TrIVD}'s \textit{zero-shot} multi-class, multi-object tracking performance~(Sec.~\ref{sec: zero-shot}). All the above videos are from \texttt{VID}~\cite{russakovsky2015vid} where no tracking annotation is available.}
	\vspace*{-0.3cm}  
	 \label{app_fig: mot_a}
\end{center}
\end{figure*}
