# Supplementary material for: Unifying Tracking and Image-Video Object Detection
Source: arXiv:2211.11077 source file (2023-11-19)
Supplement: Supplementary file 4 [file result_arxiv.tex]

\section{Additional Experimental Results}
\label{app: exp}

\begin{figure}[h]
%\vspace{0.2cm}
\begin{center}
%\hspace*{-0.55cm}  
\captionsetup{type=figure}
\resizebox{1.\linewidth}{!}{
	\begin{tikzpicture}
		\tikzstyle{myarrows}=[line width=0.6mm,draw=blue!50,-triangle 45,postaction={draw, line width=0.05mm, shorten >=0.01mm, -}]
		\tikzstyle{mylines}=[line width=0.6mm]
		% Main size box
		%\draw[thin, color = black] (10, -5) -- (-10, -5) -- (-10, 5) -- (10, 5) -- (10, -5); 
		 
   		% Denotations location control
		\pgfmathsetmacro{\dx}{3.65} 
		\pgfmathsetmacro{\dy}{2}

		\node at (-4-\dx, -6.5+3.65*\dy){\texttt{COCO}~\cite{lin2014coco}};
		\node at (-4, -6.5+3.65*\dy){\texttt{VID}~\cite{russakovsky2015vid}};
		\node at (-4+\dx, -6.5+3.65*\dy){\texttt{MOT17}~\cite{Milan2016MOT16AB}};

		\node at (-4-\dx, -6.5+3*\dy) {\includegraphics[width=3.5cm]{fig/COCO/91-341681-3_3.png}};  
		\node at (-4-\dx, -6.5+2*\dy) {\includegraphics[width=3.5cm]{fig/COCO/14-51712-2_2.png}}; 
		\node at (-4-\dx, -6.5+1*\dy) {\includegraphics[width=3.5cm]{fig/COCO/2346.png}};  
		\node at (-4-\dx, -6.5) {\includegraphics[width=3.5cm]{fig/COCO/144.png}}; 
		\node at (-4-\dx, -6.5-\dy) {\includegraphics[width=3.5cm]{fig/COCO/54592.png}}; 
		\node at (-4-\dx, -6.5-2*\dy) {\includegraphics[width=3.5cm]{fig/COCO/66771.png}}; 
		\node at (-4-\dx, -6.5-3*\dy) {\includegraphics[width=3.5cm]{fig/COCO/214753.png}}; 
		\node at (-4-\dx, -6.5-4*\dy) {\includegraphics[width=3.5cm]{fig/COCO/230008.png}};

		%\node at (-4, -6.5+3*\dy) {\includegraphics[width=3.5cm]{fig/VID/5403.jpg}}; 
		\node at (-4, -6.5+3*\dy) {\includegraphics[width=3.5cm]{fig/VID/1506.png}}; 
		\node at (-4, -6.5+2*\dy) {\includegraphics[width=3.5cm]{fig/VID/antelope2.png}};  
		\node at (-4, -6.5+1*\dy) {\includegraphics[width=3.5cm]{fig/VID/3399.png}};  
		\node at (-4, -6.5) {\includegraphics[width=3.5cm]{fig/VID/3918.png}}; 
		\node at (-4, -6.5-\dy) {\includegraphics[width=3.5cm]{fig/VID/4268.png}}; 
		\node at (-4, -6.5-2*\dy) {\includegraphics[width=3.5cm]{fig/VID/3635.png}}; 
		\node at (-4, -6.5-3*\dy) {\includegraphics[width=3.5cm]{fig/VID/antelope.png}}; 
		\node at (-4, -6.5-4*\dy) {\includegraphics[width=3.5cm]{fig/VID/5403.png}};

		\node at (-4+\dx, -6.5+3*\dy) {\includegraphics[width=3.5cm]{fig/MOT-detect/2536.png}}; 
		\node at (-4+\dx, -6.5+2*\dy) {\includegraphics[width=3.5cm]{fig/MOT-detect/550.png}}; 
		\node at (-4+\dx, -6.5+1*\dy) {\includegraphics[width=3.5cm]{fig/MOT-detect/2408.png}};  
		\node at (-4+\dx, -6.5) {\includegraphics[width=3.5cm]{fig/MOT-detect/2480.png}};  
		\node at (-4+\dx, -6.5-\dy) {\includegraphics[width=3.5cm]{fig/MOT-detect/2500.png}};  
		\node at (-4+\dx, -6.5-2*\dy) {\includegraphics[width=3.5cm]{fig/MOT-detect/228.png}};  
		\node at (-4+\dx, -6.5-3*\dy) {\includegraphics[width=3.5cm]{fig/MOT-detect/2578.png}};  
		\node at (-4+\dx, -6.5-4*\dy) {\includegraphics[width=3.5cm]{fig/MOT-detect/998.png}};

	\end{tikzpicture}
	}  
	\vspace*{-0.7cm}
    \caption{\texttt{TrIVD}'s object detection results on \texttt{COCO}, \texttt{VID}, and \texttt{MOT17}. With multi-dataset co-training, \texttt{TrIVD} detects objects (e.g., traffic lights, bicycles, motorcycles) not annotated by \texttt{MOT17}~($3^{\text{rd}}$ column).}
	 \label{app_fig: det}
\end{center}
\end{figure}

\begin{figure*}[t]
\vspace{-1.3cm}
\begin{center}
%\hspace*{-0.7cm}  
\captionsetup{type=figure}
\resizebox{0.95\linewidth}{!}{
	\begin{tikzpicture}
		\tikzstyle{myarrows}=[line width=0.6mm,draw=blue!50,-triangle 45,postaction={draw, line width=0.05mm, shorten >=0.01mm, -}]
		\tikzstyle{mylines}=[line width=0.6mm]
		% Main size box
		%\draw[thin, color = black] (10, -5) -- (-10, -5) -- (-10, 5) -- (10, 5) -- (10, -5); 
		 
   		% Global location control
		\pgfmathsetmacro{\dx}{3.6} 
		\pgfmathsetmacro{\dy}{2}
		
		\node at (-4-5.55*\dx, -6.5+9.65*\dy){\color{cb!90}$\mathbf{t}$};
		\draw [-to, line width=0.6mm, color = cb] (-4-5.55*\dx, -6.5+9.48*\dy) -- (-4-5.55*\dx, -6.5-0.51*\dy); 
		
		\node at (-4-5*\dx, -6.5+9.65*\dy){\small\textbf{\color{cb}Track} \textit{``airplane''}};
		\node at (-4-4*\dx, -6.5+9.65*\dy){\small\textbf{\color{cb}Track} \textit{``bird''}};
		\node at (-4-3*\dx, -6.5+9.65*\dy){\small\textbf{\color{cb}Track} \textit{``giant panda''}};
		\node at (-4-2*\dx, -6.5+9.65*\dy){\small\textbf{\color{cb}Track} \textit{``car''}};

		% airplane 1
		\node at (-4-5*\dx, -6.5+9*\dy) {\includegraphics[width=3.5cm]{sub/appendix/fig/airplane1/000000.JPEG}}; 
		\node at (-4-5*\dx, -6.5+8*\dy) {\includegraphics[width=3.5cm]{sub/appendix/fig/airplane1/000016.JPEG}}; 
		\node at (-4-5*\dx, -6.5+7*\dy) {\includegraphics[width=3.5cm]{sub/appendix/fig/airplane1/000030.JPEG}}; 
		\node at (-4-5*\dx, -6.5+6*\dy) {\includegraphics[width=3.5cm]{sub/appendix/fig/airplane1/000045.JPEG}}; 
		\node at (-4-5*\dx, -6.5+5*\dy) {\includegraphics[width=3.5cm]{sub/appendix/fig/airplane1/000056.JPEG}}; 
		\node at (-4-5*\dx, -6.5+4*\dy) {\includegraphics[width=3.5cm]{sub/appendix/fig/airplane1/000065.JPEG}}; 
		\node at (-4-5*\dx, -6.5+3*\dy) {\includegraphics[width=3.5cm]{sub/appendix/fig/airplane1/000076.JPEG}}; 
		\node at (-4-5*\dx, -6.5+2*\dy) {\includegraphics[width=3.5cm]{sub/appendix/fig/airplane1/000086.JPEG}}; 
		\node at (-4-5*\dx, -6.5+1*\dy) {\includegraphics[width=3.5cm]{sub/appendix/fig/airplane1/000105.JPEG}}; 
		\node at (-4-5*\dx, -6.5) {\includegraphics[width=3.5cm]{sub/appendix/fig/airplane1/000127.JPEG}};

		% birds
		\node at (-4-4*\dx, -6.5+9*\dy) {\includegraphics[width=3.5cm]{sub/appendix/fig/birds/000000.JPEG}}; 
		\node at (-4-4*\dx, -6.5+8*\dy) {\includegraphics[width=3.5cm]{sub/appendix/fig/birds/000081.JPEG}}; 
		\node at (-4-4*\dx, -6.5+7*\dy) {\includegraphics[width=3.5cm]{sub/appendix/fig/birds/000124.JPEG}}; 
		\node at (-4-4*\dx, -6.5+6*\dy) {\includegraphics[width=3.5cm]{sub/appendix/fig/birds/000167.JPEG}}; 
		\node at (-4-4*\dx, -6.5+5*\dy) {\includegraphics[width=3.5cm]{sub/appendix/fig/birds/000177.JPEG}}; 
		\node at (-4-4*\dx, -6.5+4*\dy) {\includegraphics[width=3.5cm]{sub/appendix/fig/birds/000190.JPEG}}; 
		\node at (-4-4*\dx, -6.5+3*\dy) {\includegraphics[width=3.5cm]{sub/appendix/fig/birds/000197.JPEG}}; 
		\node at (-4-4*\dx, -6.5+2*\dy) {\includegraphics[width=3.5cm]{sub/appendix/fig/birds/000207.JPEG}}; 
		\node at (-4-4*\dx, -6.5+1*\dy) {\includegraphics[width=3.5cm]{sub/appendix/fig/birds/000232.JPEG}}; 
		\node at (-4-4*\dx, -6.5) {\includegraphics[width=3.5cm]{sub/appendix/fig/birds/000257.JPEG}};

		% pandas
		\node at (-4-3*\dx, -6.5+9*\dy) {\includegraphics[width=3.5cm]{sub/appendix/fig/pandas/000000.JPEG}}; 
		\node at (-4-3*\dx, -6.5+8*\dy) {\includegraphics[width=3.5cm]{sub/appendix/fig/pandas/000016.JPEG}}; 
		\node at (-4-3*\dx, -6.5+7*\dy) {\includegraphics[width=3.5cm]{sub/appendix/fig/pandas/000044.JPEG}}; 
		\node at (-4-3*\dx, -6.5+6*\dy) {\includegraphics[width=3.5cm]{sub/appendix/fig/pandas/000058.JPEG}}; 
		\node at (-4-3*\dx, -6.5+5*\dy) {\includegraphics[width=3.5cm]{sub/appendix/fig/pandas/000091.JPEG}}; 
		\node at (-4-3*\dx, -6.5+4*\dy) {\includegraphics[width=3.5cm]{sub/appendix/fig/pandas/000094.JPEG}}; 
		\node at (-4-3*\dx, -6.5+3*\dy) {\includegraphics[width=3.5cm]{sub/appendix/fig/pandas/000115.JPEG}}; 
		\node at (-4-3*\dx, -6.5+2*\dy) {\includegraphics[width=3.5cm]{sub/appendix/fig/pandas/000140.JPEG}}; 
		\node at (-4-3*\dx, -6.5+1*\dy) {\includegraphics[width=3.5cm]{sub/appendix/fig/pandas/000164.JPEG}}; 
		\node at (-4-3*\dx, -6.5) {\includegraphics[width=3.5cm]{sub/appendix/fig/pandas/000191.JPEG}};

		% car
		\node at (-4-2*\dx, -6.5+9*\dy) {\includegraphics[width=3.5cm]{sub/appendix/fig/car/000000.JPEG}}; 
		\node at (-4-2*\dx, -6.5+8*\dy) {\includegraphics[width=3.5cm]{sub/appendix/fig/car/000012.JPEG}}; 
		\node at (-4-2*\dx, -6.5+7*\dy) {\includegraphics[width=3.5cm]{sub/appendix/fig/car/000019.JPEG}}; 
		\node at (-4-2*\dx, -6.5+6*\dy) {\includegraphics[width=3.5cm]{sub/appendix/fig/car/000030.JPEG}}; 
		\node at (-4-2*\dx, -6.5+5*\dy) {\includegraphics[width=3.5cm]{sub/appendix/fig/car/000037.JPEG}}; 
		\node at (-4-2*\dx, -6.5+4*\dy) {\includegraphics[width=3.5cm]{sub/appendix/fig/car/000042.JPEG}}; 
		\node at (-4-2*\dx, -6.5+3*\dy) {\includegraphics[width=3.5cm]{sub/appendix/fig/car/000047.JPEG}}; 
		\node at (-4-2*\dx, -6.5+2*\dy) {\includegraphics[width=3.5cm]{sub/appendix/fig/car/000055.JPEG}}; 
		\node at (-4-2*\dx, -6.5+1*\dy) {\includegraphics[width=3.5cm]{sub/appendix/fig/car/000067.JPEG}}; 
		\node at (-4-2*\dx, -6.5) {\includegraphics[width=3.5cm]{sub/appendix/fig/car/000092.JPEG}};

	\end{tikzpicture}
	}  
	\vspace*{-0.4cm}
    \caption{Visualizations on \texttt{TrIVD}'s \textit{zero-shot} multi-class, multi-object tracking performance~(Sec.~\ref{sec: zero-shot}). All the above videos are from \texttt{VID}~\cite{russakovsky2015vid} where no tracking annotation is available.}
	\vspace*{-0.3cm}  
	 \label{app_fig: mot_a}
\end{center}
\end{figure*}

\begin{figure*}[t]
\vspace{-1.3cm}
\begin{center}
%\hspace*{-0.7cm}  
\captionsetup{type=figure}
\resizebox{0.95\linewidth}{!}{
	\begin{tikzpicture}
		\tikzstyle{myarrows}=[line width=0.6mm,draw=blue!50,-triangle 45,postaction={draw, line width=0.05mm, shorten >=0.01mm, -}]
		\tikzstyle{mylines}=[line width=0.6mm]
		% Main size box
		%\draw[thin, color = black] (10, -5) -- (-10, -5) -- (-10, 5) -- (10, 5) -- (10, -5); 
		 
   		% Global location control
		\pgfmathsetmacro{\dx}{3.6} 
		\pgfmathsetmacro{\dy}{2}
		
		\node at (-4-5.55*\dx, -6.5+9.65*\dy){\color{cb!90}$\mathbf{t}$};
		\draw [-to, line width=0.6mm, color = cb] (-4-5.55*\dx, -6.5+9.48*\dy) -- (-4-5.55*\dx, -6.5-0.51*\dy); 
		
		\node at (-4-5*\dx, -6.5+9.65*\dy){\small\textbf{\color{cb}Track} \textit{``airplane''}};
		\node at (((-4-4.02*\dx, -6.5+9.65*\dy){\small\textbf{\color{cb}Track} \textit{``horse''}};
		\node at ((-4-3.045*\dx, -6.5+9.65*\dy){\small\textbf{\color{cb}Track} \textit{``car''}};
		\node at (-4-2.045*\dx, -6.5+9.65*\dy){\small\textbf{\color{cb}Track} \textit{``bicycle''}};

		% horse
		\node at (((-4-4.02*\dx, -6.5+9*\dy) {\includegraphics[width=3.35cm]{sub/appendix/fig/horse/0001.jpg}}; 
		\node at (((-4-4.02*\dx, -6.5+8*\dy) {\includegraphics[width=3.35cm]{sub/appendix/fig/horse/0002.jpg}}; 
		\node at (((-4-4.02*\dx, -6.5+7*\dy) {\includegraphics[width=3.35cm]{sub/appendix/fig/horse/0003.jpg}}; 
		\node at (((-4-4.02*\dx, -6.5+6*\dy) {\includegraphics[width=3.35cm]{sub/appendix/fig/horse/0004.jpg}}; 
		\node at (((-4-4.02*\dx, -6.5+5*\dy) {\includegraphics[width=3.35cm]{sub/appendix/fig/horse/0005.jpg}}; 
		\node at (((-4-4.02*\dx, -6.5+4*\dy) {\includegraphics[width=3.35cm]{sub/appendix/fig/horse/0006.jpg}}; 
		\node at (((-4-4.02*\dx, -6.5+3*\dy) {\includegraphics[width=3.35cm]{sub/appendix/fig/horse/0007.jpg}}; 
		\node at (((-4-4.02*\dx, -6.5+2*\dy) {\includegraphics[width=3.35cm]{sub/appendix/fig/horse/0008.jpg}}; 
		\node at (((-4-4.02*\dx, -6.5+1*\dy) {\includegraphics[width=3.35cm]{sub/appendix/fig/horse/0009.jpg}}; 
		\node at (((-4-4.02*\dx, -6.5) {\includegraphics[width=3.35cm]{sub/appendix/fig/horse/0010.jpg}};

		% cars
		\node at ((-4-3.045*\dx, -6.5+9*\dy) {\includegraphics[width=3.5cm]{sub/appendix/fig/cars/000000.JPEG}}; 
		\node at ((-4-3.045*\dx, -6.5+8*\dy) {\includegraphics[width=3.5cm]{sub/appendix/fig/cars/000009.JPEG}}; 
		\node at ((-4-3.045*\dx, -6.5+7*\dy) {\includegraphics[width=3.5cm]{sub/appendix/fig/cars/000019.JPEG}}; 
		\node at ((-4-3.045*\dx, -6.5+6*\dy) {\includegraphics[width=3.5cm]{sub/appendix/fig/cars/000029.JPEG}}; 
		\node at ((-4-3.045*\dx, -6.5+5*\dy) {\includegraphics[width=3.5cm]{sub/appendix/fig/cars/000035.JPEG}}; 
		\node at ((-4-3.045*\dx, -6.5+4*\dy) {\includegraphics[width=3.5cm]{sub/appendix/fig/cars/000042.JPEG}}; 
		\node at ((-4-3.045*\dx, -6.5+3*\dy) {\includegraphics[width=3.5cm]{sub/appendix/fig/cars/000047.JPEG}}; 
		\node at ((-4-3.045*\dx, -6.5+2*\dy) {\includegraphics[width=3.5cm]{sub/appendix/fig/cars/000051.JPEG}}; 
		\node at ((-4-3.045*\dx, -6.5+1*\dy) {\includegraphics[width=3.5cm]{sub/appendix/fig/cars/000056.JPEG}}; 
		\node at ((-4-3.045*\dx, -6.5) {\includegraphics[width=3.5cm]{sub/appendix/fig/cars/000058.JPEG}};

		% airplane2
		\node at (-4-5*\dx, -6.5+9*\dy) {\includegraphics[width=3.5cm]{sub/appendix/fig/airplane2/000000.JPEG}}; 
		\node at (-4-5*\dx, -6.5+8*\dy) {\includegraphics[width=3.5cm]{sub/appendix/fig/airplane2/000009.JPEG}}; 
		\node at (-4-5*\dx, -6.5+7*\dy) {\includegraphics[width=3.5cm]{sub/appendix/fig/airplane2/000021.JPEG}}; 
		\node at (-4-5*\dx, -6.5+6*\dy) {\includegraphics[width=3.5cm]{sub/appendix/fig/airplane2/000038.JPEG}}; 
		\node at (-4-5*\dx, -6.5+5*\dy) {\includegraphics[width=3.5cm]{sub/appendix/fig/airplane2/000044.JPEG}}; 
		\node at (-4-5*\dx, -6.5+4*\dy) {\includegraphics[width=3.5cm]{sub/appendix/fig/airplane2/000050.JPEG}}; 
		\node at (-4-5*\dx, -6.5+3*\dy) {\includegraphics[width=3.5cm]{sub/appendix/fig/airplane2/000059.JPEG}}; 
		\node at (-4-5*\dx, -6.5+2*\dy) {\includegraphics[width=3.5cm]{sub/appendix/fig/airplane2/000067.JPEG}}; 
		\node at (-4-5*\dx, -6.5+1*\dy) {\includegraphics[width=3.5cm]{sub/appendix/fig/airplane2/000076.JPEG}}; 
		\node at (-4-5*\dx, -6.5) {\includegraphics[width=3.5cm]{sub/appendix/fig/airplane2/000084.JPEG}};

		% bicycle
		\node at (-4-2.045*\dx, -6.5+9*\dy) {\includegraphics[width=3.5cm]{sub/appendix/fig/bicycles/000021.JPEG}}; 
		\node at (-4-2.045*\dx, -6.5+8*\dy) {\includegraphics[width=3.5cm]{sub/appendix/fig/bicycles/000027.JPEG}}; 
		\node at (-4-2.045*\dx, -6.5+7*\dy) {\includegraphics[width=3.5cm]{sub/appendix/fig/bicycles/000036.JPEG}}; 
		\node at (-4-2.045*\dx, -6.5+6*\dy) {\includegraphics[width=3.5cm]{sub/appendix/fig/bicycles/000044.JPEG}}; 
		\node at (-4-2.045*\dx, -6.5+5*\dy) {\includegraphics[width=3.5cm]{sub/appendix/fig/bicycles/000055.JPEG}}; 
		\node at (-4-2.045*\dx, -6.5+4*\dy) {\includegraphics[width=3.5cm]{sub/appendix/fig/bicycles/000064.JPEG}}; 
		\node at (-4-2.045*\dx, -6.5+3*\dy) {\includegraphics[width=3.5cm]{sub/appendix/fig/bicycles/000067.JPEG}}; 
		\node at (-4-2.045*\dx, -6.5+2*\dy) {\includegraphics[width=3.5cm]{sub/appendix/fig/bicycles/000074.JPEG}}; 
		\node at (-4-2.045*\dx, -6.5+1*\dy) {\includegraphics[width=3.5cm]{sub/appendix/fig/bicycles/000083.JPEG}}; 
		\node at (-4-2.045*\dx, -6.5) {\includegraphics[width=3.5cm]{sub/appendix/fig/bicycles/000104.JPEG}};

	\end{tikzpicture}
	}  
	\vspace*{-0.4cm}
    \caption{Visualizations on \texttt{TrIVD}'s \textit{zero-shot} multi-class, multi-object tracking performance~(Sec.~\ref{sec: zero-shot}). All the above videos are from \texttt{VID}~\cite{russakovsky2015vid} where no tracking annotation is available. In the last column, we show a failure case where the model recognizes the ``blue-box'' bicycle as a new track (``green-box'') when it re-enters the scene, due to the significant pose and camera view changes.}
	\vspace*{-0.3cm}  
	 \label{app_fig: mot_b}
\end{center}
\end{figure*}

%%%%%%%%%%%%%
%%%%%%%%%%%%%

\subsection{Unified Image-Video Backbone Design Comparisons}
\label{app: omnivore}

%%%%%%%%%%%%%
%%%%%%%%%%%%%

\subsection{Zero-shot Multi-object Tracking}
\label{app: mot}

In Fig.~\ref{app_fig: mot_a} and Fig.~\ref{app_fig: mot_b}, we present more complete zero-shot multi-object tracking results from \texttt{TrIVD}, in addition to Fig.~\ref{fig: showcase} and Fig.~\ref{fig: mot} in the main paper.

%%%%%%%%%%%%%
%%%%%%%%%%%%%

\subsection{Cross-dataset Detection}
\label{app: det}

We provide more cross-dataset detection results in Fig.~\ref{app_fig: det} on all the three experimented datasets (\texttt{COCO}~\cite{lin2014coco}, \texttt{VID}~\cite{russakovsky2015vid}, \texttt{MOT}~\cite{Milan2016MOT16AB}) in addition to Fig.~\ref{fig: showcase} and Fig.~\ref{fig: det} in the main paper.
